# Supplementary material for: Fast Compact Laser Shutter Using a Direct Current Motor and 3D Printing
Source: arXiv:1509.01566 ancillary file (2015-09-21)
Supplement: Supplementary file 1 [file 2DShutter.PDF]

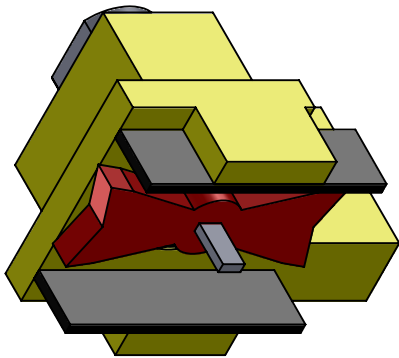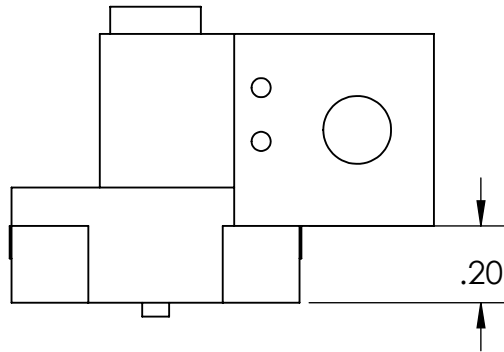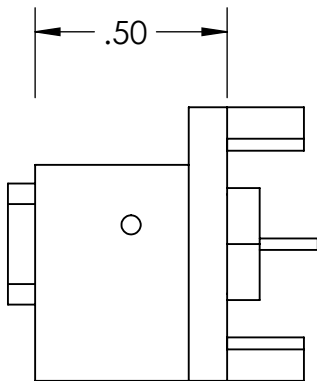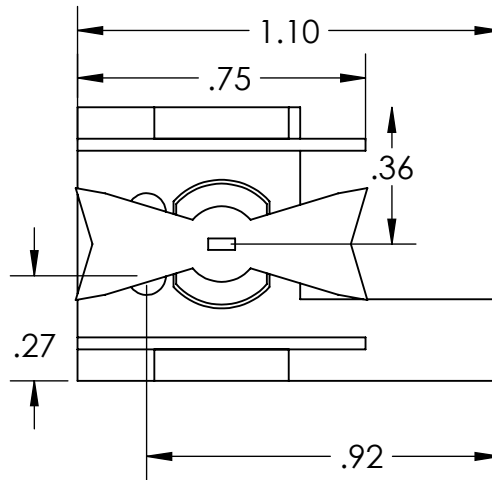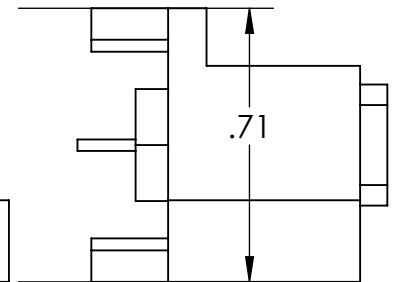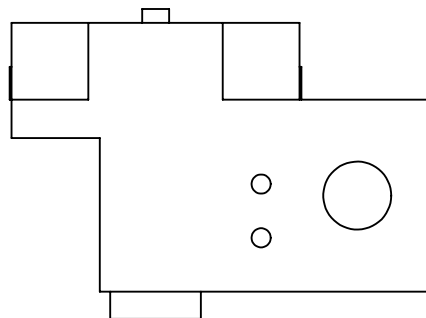

**PROPRIETARY AND CONFIDENTIAL**  
 THE INFORMATION CONTAINED  
 HEREIN IS THE SOLE PROPERTY OF  
 <INSERT COMPANY NAME>  
 REPRODUCTION IN PART OR AS A WHOLE  
 WITHOUT THE WRITTEN PERMISSION OF  
 <INSERT COMPANY NAME HERE> IS  
 PROHIBITED.

**SolidWorks Student Edition.**  
**For Academic Use Only.**

|                                   |         |                                                                                                                                            |                  |                               |         |              |  |           |
|-----------------------------------|---------|--------------------------------------------------------------------------------------------------------------------------------------------|------------------|-------------------------------|---------|--------------|--|-----------|
|                                   |         | DIMENSIONS ARE IN INCHES<br>TOLERANCES:<br>FRACTIONAL ±<br>ANGULAR: MACH ±    BEND ±<br>TWO PLACE DECIMAL    ±<br>THREE PLACE DECIMAL    ± | NAME             | DATE                          |         |              |  |           |
|                                   |         |                                                                                                                                            | DRAWN            | AK                            |         |              |  | 11/3/2014 |
|                                   |         |                                                                                                                                            | CHECKED          |                               |         |              |  |           |
|                                   |         |                                                                                                                                            | ENG APPR.        |                               |         |              |  |           |
|                                   |         |                                                                                                                                            | MFG APPR.        |                               |         |              |  |           |
| Student Edition.<br>Mic Use Only. |         |                                                                                                                                            | Q.A.             |                               |         |              |  |           |
|                                   |         |                                                                                                                                            | COMMENTS:        |                               |         |              |  |           |
| NEXT ASSY                         | USED ON | FINISH                                                                                                                                     |                  |                               |         |              |  |           |
| APPLICATION                       |         | DO NOT SCALE DRAWING                                                                                                                       |                  |                               |         |              |  |           |
|                                   |         |                                                                                                                                            | SIZE<br><b>A</b> | DWG. NO.<br><b>Assembled6</b> |         | REV.         |  |           |
|                                   |         |                                                                                                                                            | SCALE:2:1        |                               | WEIGHT: | SHEET 1 OF 3 |  |           |

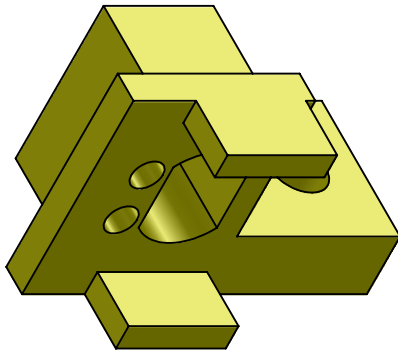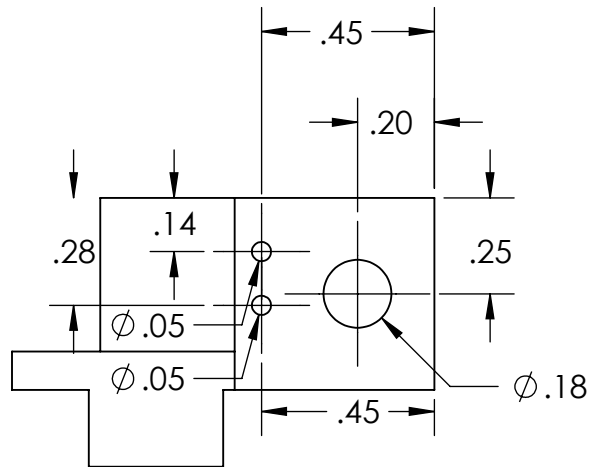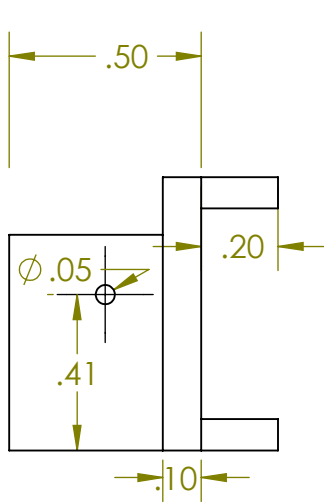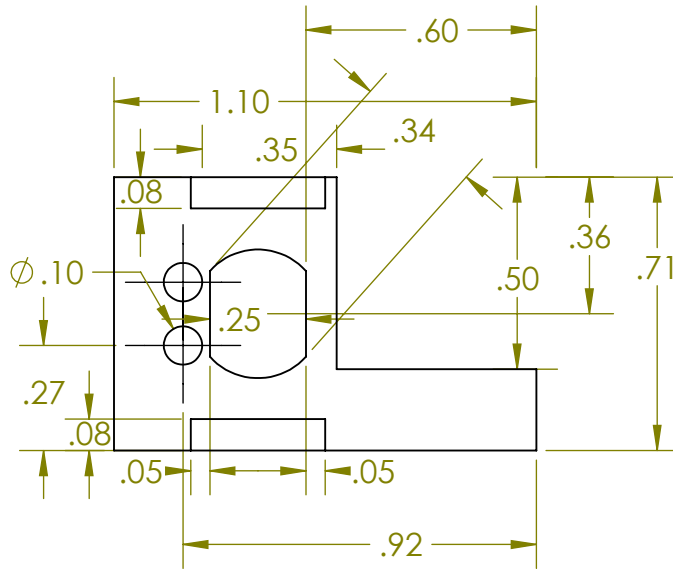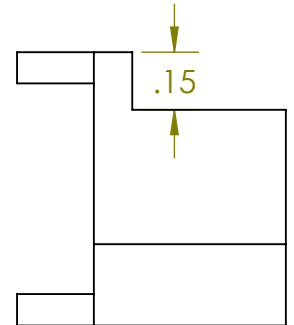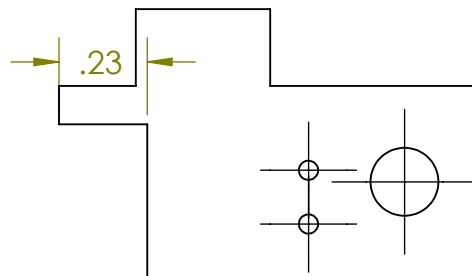

|                                                                                                                                                                                                                                                          |  |                                                                                                                                                       |        |           |      |                                                                         |           |
|----------------------------------------------------------------------------------------------------------------------------------------------------------------------------------------------------------------------------------------------------------|--|-------------------------------------------------------------------------------------------------------------------------------------------------------|--------|-----------|------|-------------------------------------------------------------------------|-----------|
| <b>PROPRIETARY AND CONFIDENTIAL</b><br>THE INFORMATION CONTAINED HEREIN IS THE SOLE PROPERTY OF<br><INSERT COMPANY NAME HERE><br>REPRODUCTION IN PART OR AS A WHOLE<br>WITHOUT THE WRITTEN PERMISSION OF<br><INSERT COMPANY NAME HERE> IS<br>PROHIBITED. |  | DIMENSIONS ARE IN INCHES<br>TOLERANCES:<br>FRACTIONAL $\pm$<br>ANGULAR: MACH $\pm$ BEND $\pm$<br>TWO PLACE DECIMAL $\pm$<br>THREE PLACE DECIMAL $\pm$ |        | NAME      | DATE | SIZE DWG. NO. <b>Assembled6</b> REV.<br>SCALE: 2:1 WEIGHT: SHEET 2 OF 3 |           |
|                                                                                                                                                                                                                                                          |  |                                                                                                                                                       |        | DRAWN     | AK   |                                                                         | 6/30/2014 |
|                                                                                                                                                                                                                                                          |  |                                                                                                                                                       |        | CHECKED   |      |                                                                         |           |
|                                                                                                                                                                                                                                                          |  |                                                                                                                                                       |        | ENG APPR. |      |                                                                         |           |
|                                                                                                                                                                                                                                                          |  |                                                                                                                                                       |        | MFG APPR. |      |                                                                         |           |
| NEXT ASSY                                                                                                                                                                                                                                                |  | USED ON                                                                                                                                               | FINISH | COMMENTS: |      |                                                                         |           |
| APPLICATION                                                                                                                                                                                                                                              |  | DO NOT SCALE DRAWING                                                                                                                                  |        |           |      |                                                                         |           |

**SolidWorks Student Edition.**  
**For Academic Use Only.**

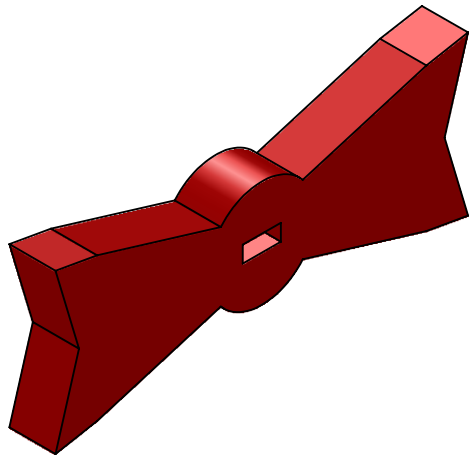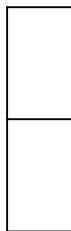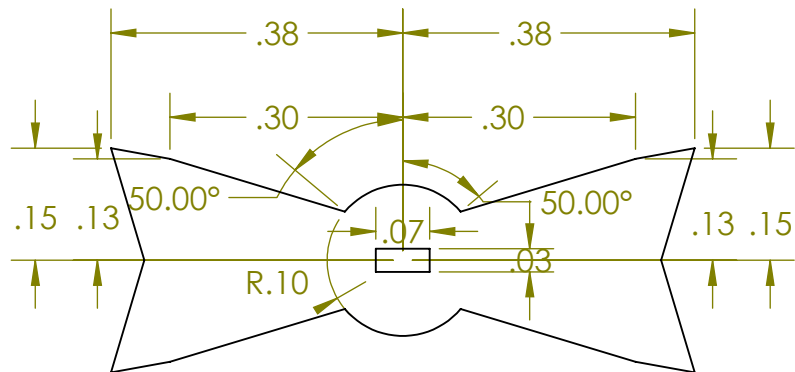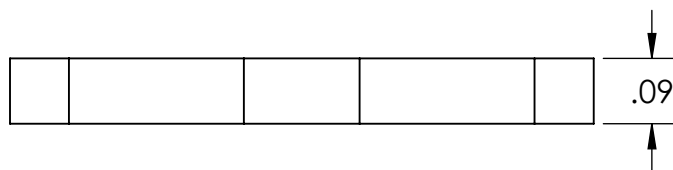

|                                                                                                                                                                                                                                       |             |         |                                                                                                                                                       |           |      |                  |           |            |      |  |
|---------------------------------------------------------------------------------------------------------------------------------------------------------------------------------------------------------------------------------------|-------------|---------|-------------------------------------------------------------------------------------------------------------------------------------------------------|-----------|------|------------------|-----------|------------|------|--|
| <b>PROPRIETARY AND CONFIDENTIAL</b><br>THE INFORMATION CONTAINED HEREIN IS THE SOLE PROPERTY OF <INSERT COMPANY NAME>. REPRODUCTION IN PART OR AS A WHOLE WITHOUT THE WRITTEN PERMISSION OF <INSERT COMPANY NAME HERE> IS PROHIBITED. |             |         | DIMENSIONS ARE IN INCHES<br>TOLERANCES:<br>FRACTIONAL $\pm$<br>ANGULAR: MACH $\pm$ BEND $\pm$<br>TWO PLACE DECIMAL $\pm$<br>THREE PLACE DECIMAL $\pm$ | NAME      | DATE | SIZE<br><b>A</b> | DWG. NO.  | Assembled6 | REV. |  |
|                                                                                                                                                                                                                                       |             |         |                                                                                                                                                       | DRAWN     | AK   |                  | 9/12/2014 |            |      |  |
|                                                                                                                                                                                                                                       |             |         |                                                                                                                                                       | CHECKED   |      |                  |           |            |      |  |
|                                                                                                                                                                                                                                       |             |         |                                                                                                                                                       | ENG APPR. |      |                  |           |            |      |  |
|                                                                                                                                                                                                                                       |             |         |                                                                                                                                                       | MFG APPR. |      |                  |           |            |      |  |
|                                                                                                                                                                                                                                       |             |         |                                                                                                                                                       | Q.A.      |      |                  |           |            |      |  |
|                                                                                                                                                                                                                                       |             |         |                                                                                                                                                       | COMMENTS: |      |                  |           |            |      |  |
|                                                                                                                                                                                                                                       | NEXT ASSY   | USED ON | FINISH                                                                                                                                                |           |      |                  |           |            |      |  |
|                                                                                                                                                                                                                                       | APPLICATION |         | DO NOT SCALE DRAWING                                                                                                                                  |           |      |                  |           |            |      |  |
| SCALE: 4:1      WEIGHT:      SHEET 3 OF 3                                                                                                                                                                                             |             |         |                                                                                                                                                       |           |      |                  |           |            |      |  |

**SolidWorks Student Edition.**  
**For Academic Use Only.**
