# Supplementary material for: Fast Compact Laser Shutter Using a Direct Current Motor and 3D Printing
Source: arXiv:1509.01566 ancillary file (2015-09-21)
Supplement: Supplementary file 2 [file Instructions.pdf]

# FAST COMPACT LASER SHUTTER USING A DIRECT CURRENT MOTOR AND 3D PRINTING

---

## SHUTTER ASSEMBLY INSTRUCTIONS

SUPPLEMENT TO ARXIV:1509.01566

---

Grace H. Zhang, Boris Braverman, Akio Kawasaki, Vladan Vuletić

MIT-HARVARD CENTER FOR ULTRACOLD ATOMS  
RESEARCH LABORATORY OF ELECTRONICS  
MASSACHUSETTS INSTITUTE OF TECHNOLOGY

September 20, 2015

# 1 Parts List

Table 1: Materials for a single shutter unit.

| Quantity | Digikey Part #<br>or File Name | Manufacturer                     | Description                 |
|----------|--------------------------------|----------------------------------|-----------------------------|
| 1        | P14350-ND                      | NMB Technologies<br>(PNN7RE08JD) | Brushed DC Motor (3V)       |
| 1        | Body                           |                                  | 3D printed body             |
| 1        | Blade                          |                                  | 3D printed blade            |
|          |                                |                                  | Neoprene Rubber (1/32" 80A) |

It is recommended that the specifications for these components be followed closely as: 1. The design of the 3D printed body in the CAD file `Body.SLDPRT` is made to accommodate the specified DC motor (NMB Technologies PNN7RE08JD). 2. The thickness and hardness specified for the Neoprene rubber have shown to deliver optimal performance during testing.

CAD files for 3D printing are provided in the following formats: `.DXF`, `.STEP`, `.STL`. The original SOLIDWORKS files and a 2D drawing of the parts and assembly are available under `Blade.SLDPRT`, `Body.SLDPRT`, `Assembly6.SLDASM`, and `2DShutter.PDF`.

Table 2: Materials for a single shutter driver. Each driver drives four shutters.

| Quantity | Digikey Part #<br>or File Name | Manufacturer                           | Description                                |
|----------|--------------------------------|----------------------------------------|--------------------------------------------|
| 4        | TA8428KOS-ND                   | Toshiba Semiconductor<br>(TA8428KS)    | Full Bridge Driver IC                      |
| 1        | 296-14876-1-ND                 | Texas Instruments<br>(SN74LS06DR)      | IC Logic Inverter                          |
| 4        | P1181-ND                       | Panasonic Electronic<br>(ECE-A1EN221U) | Bipolar capacitor<br>(220 $\mu$ F, 25V)    |
| 4        | 220YCT-ND                      | Yageo<br>(FMP200FRF52-220R)            | Resistor (220 $\Omega$ , 2W)               |
| 1        | <code>Shutter.brd</code>       | Alberta Printed Circuits               | Single-sided PCB<br>(2.00" $\times$ 2.05") |

The resistor, capacitor, and PCB can be manufactured by other companies; performance of the shutter should not vary as long as the relevant values of these components stay unchanged.

## 2 Shutter Unit

Basic assembly instructions are as follows. Specific parameters, such as the dimensions of the rubber flaps, can be slightly adjusted if desired.

1. 3D print the shutter body and shutter blade using the corresponding CAD files: **Body.SLDPRT** and **Blade.SLDPRT**. An assembly file for the entire shutter, labeled in Fig. 1a, is also included under **Assembly.SLDASM** for reference.
2. Cut two  $0.2'' \times 0.78''$  pieces of neoprene rubber and glue each symmetrically, as shown in Fig. 1a, onto the upper support and the lower support.
3. Flatten the motor axle in a vise from a  $0.040'' \times 0.040''$  cylinder into a rectangular shape that is around  $0.020''$  thick and about  $0.060''$  long, as seen in Fig. 1a. Best results are achieved by using hardened steel blocks clamped in an end mill vise, and crushing the motor axle until the shorter dimension of the axle cross section reaches about  $1/2$ – $2/3$  of its original thickness.
4. Insert the DC motor into the cavity of the 3D printed shutter body and secure in place with superglue. The front surface of the motor from which the axle extends should be approximately flush with the surface of the plastic.
5. Insert the flattened axle of the DC motor into the hole at the center of the 3D printed shutter blade and secure in place with superglue.
6. Solder connections to the DC motor as required.

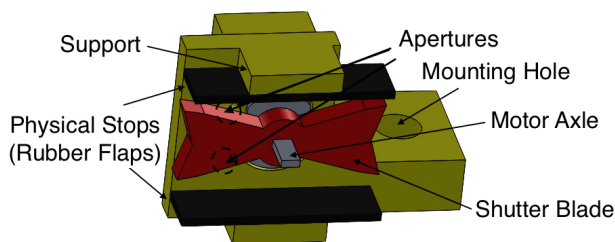

(a) CAD file of the entire shutter assembly with body, blade, motor, and rubber flaps.

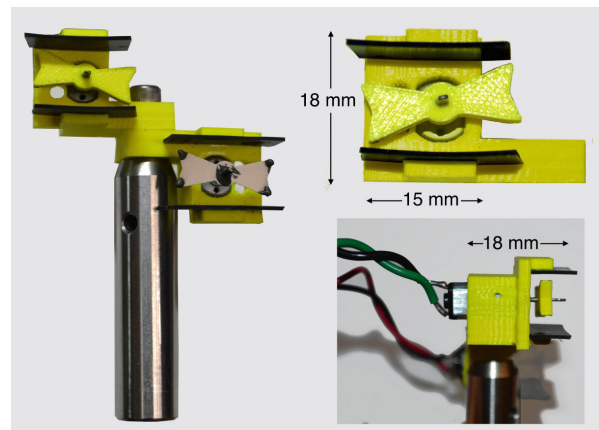

(b) Photographed shutters, with plastic blade and metal blade, stacked on an optical post.

### 3 Shutter Driver

Each shutter driver drives four separate shutters. The PCB circuit board can be found under `Shutter.brd`, with the electronic components listed in Table 2. Files for the component side, solder side, and drill data for Numerical Control (NC) drill machine will generally be needed when ordering printed circuited boards, and are available under `Shutter.cmp`, `Shutter.sol`, `Shutter.drd`. The electronic circuit is explained in detail in the paper (arXiv:1509.01566), and external connections can be wired as needed as shown in Fig. 2c.

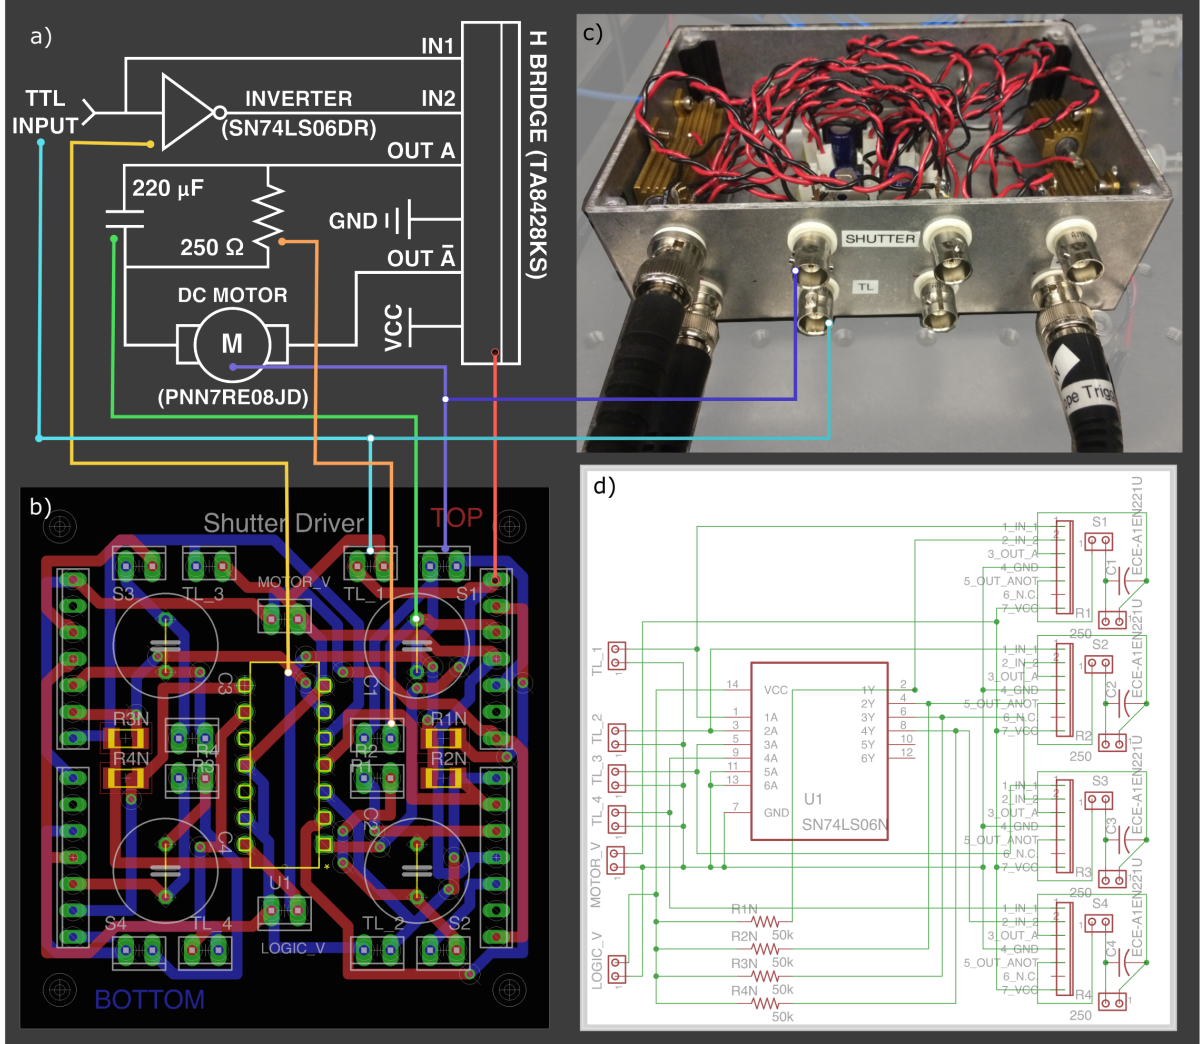

Figure 2: Assembly connections between a) Simple circuit schematic for a single shutter as shown in the paper, b) the PCB board of the driver for 4 shutters, d) its corresponding circuit schematic, and c) the electronic box with the constructed circuit shutter driver and external connections to the shutter and the input TTL signal.
